# Supplementary material for: First-principles study of defects at $\Sigma3$ grain boundaries in CuGaSe$_2$
Source: arXiv:2103.10704 ancillary file (2021-03-19)
Supplement: Supplementary file 1 [file SupplementaryData.pdf]

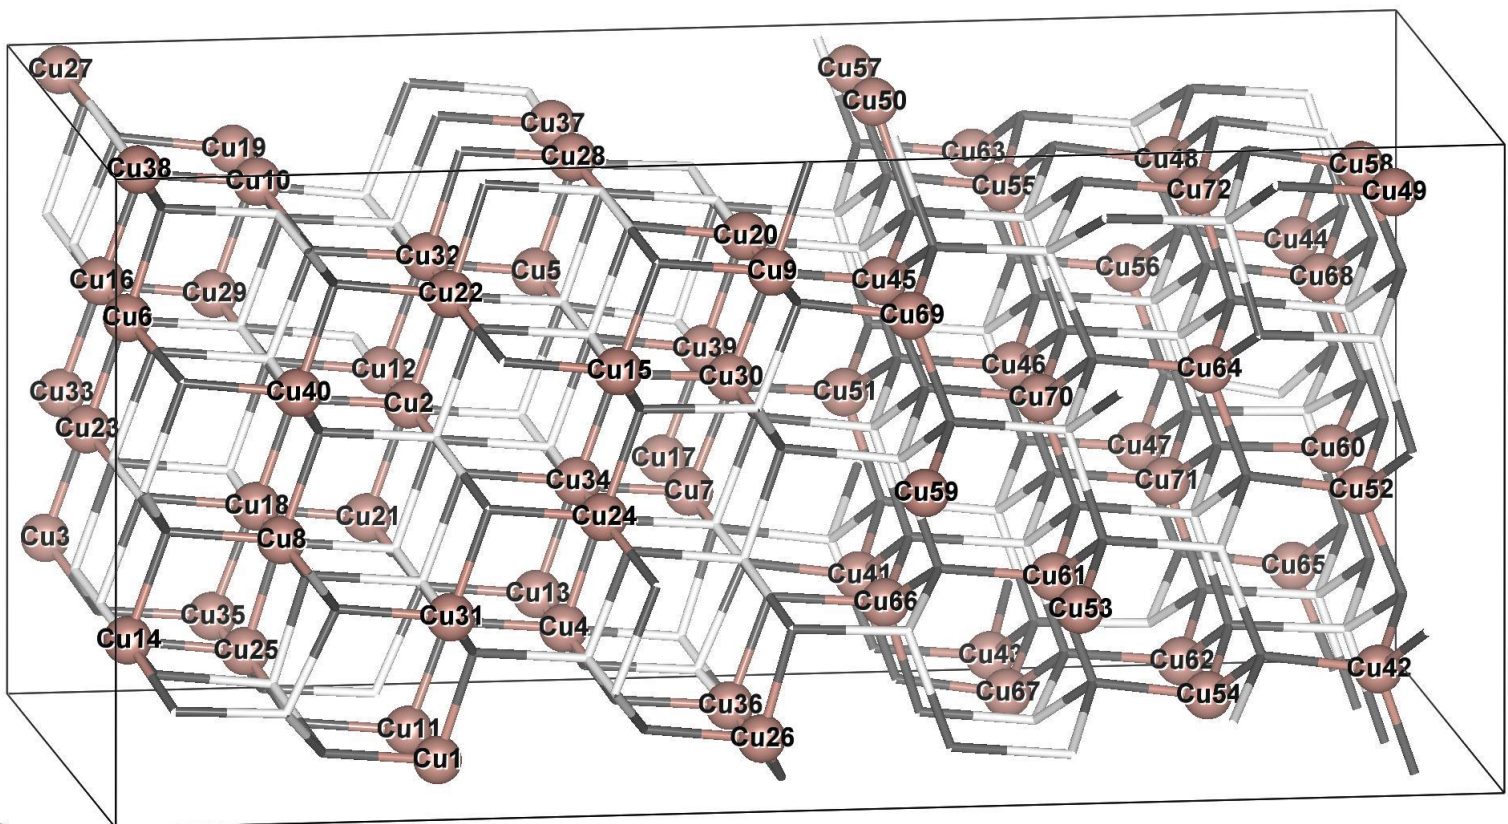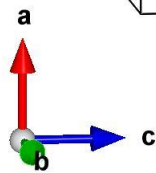

Above: Positions of the Cu atoms in the GB supercell as numbered in the following pages. For clarity, the Ga and Se atoms are not shown. To the right: Lower panel of Fig. 1 in the main article, shown for comparison.

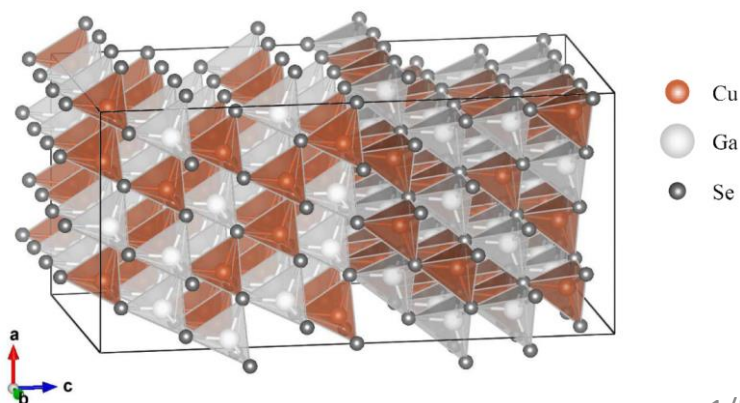

# Cu vacancies: $V_{\text{Cu}}$

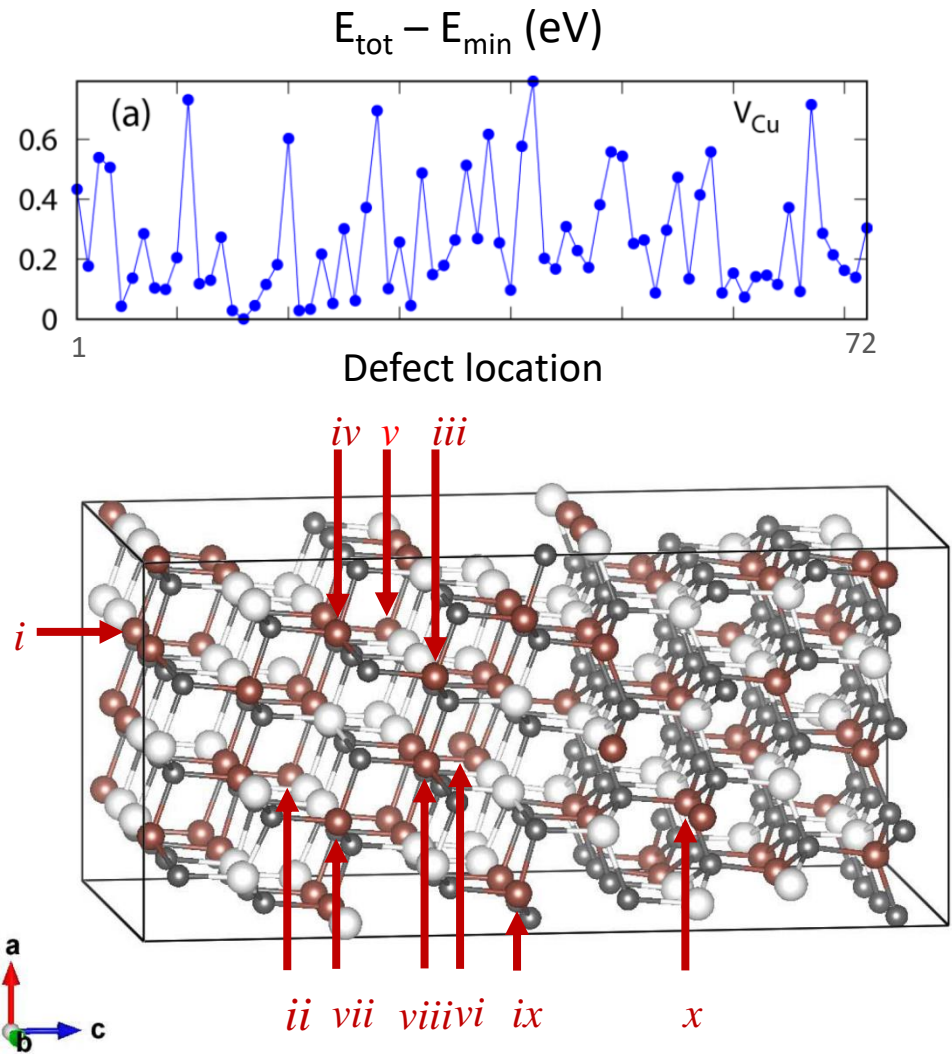

Upper panel: Total energies for  $V_{\text{Cu}}$  at the different possible locations  
 Lower panel: Locations corresponding to the 10 lowest energy  $V_{\text{Cu}}$  defects

## Ga at Cu defects: $\text{Ga}_{\text{Cu}}$

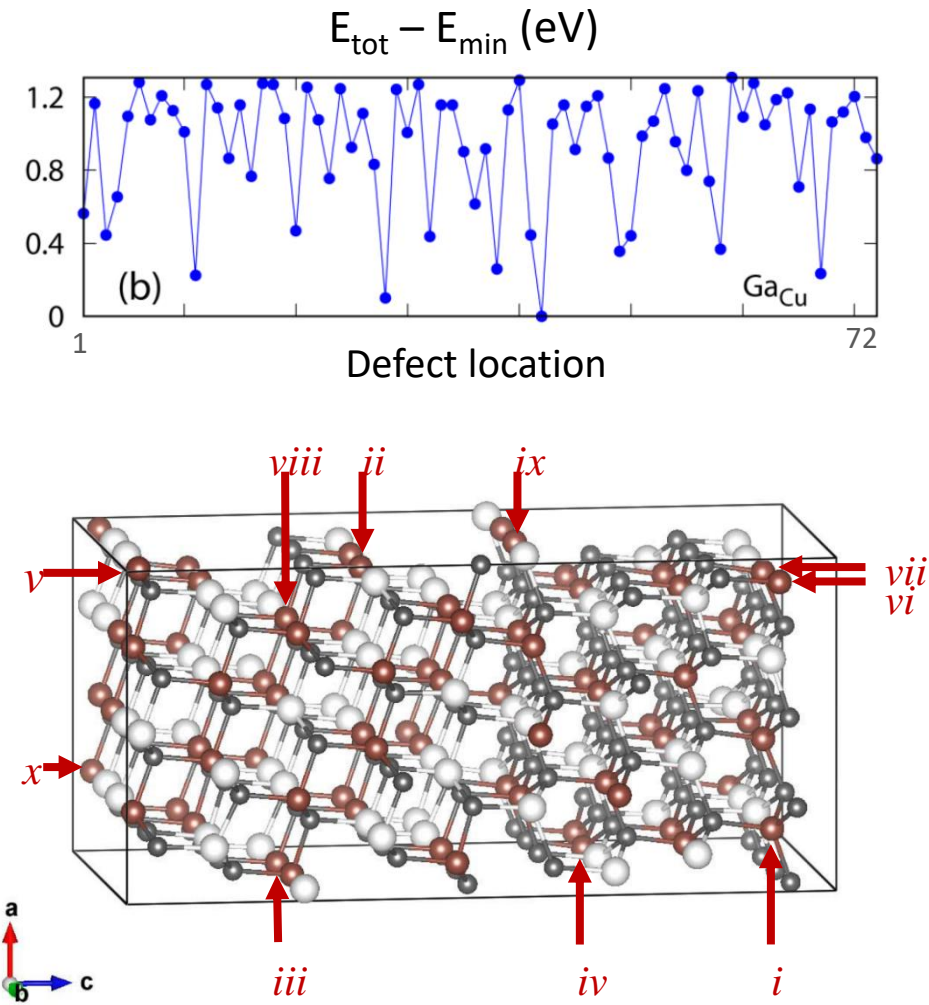

Upper panel: Total energies for  $\text{Ga}_{\text{Cu}}$  at the different possible locations  
Lower panel: Locations corresponding to the 10 lowest energy  $\text{Ga}_{\text{Cu}}$  defects

## Na at Cu impurities: $\text{Na}_{\text{Cu}}$

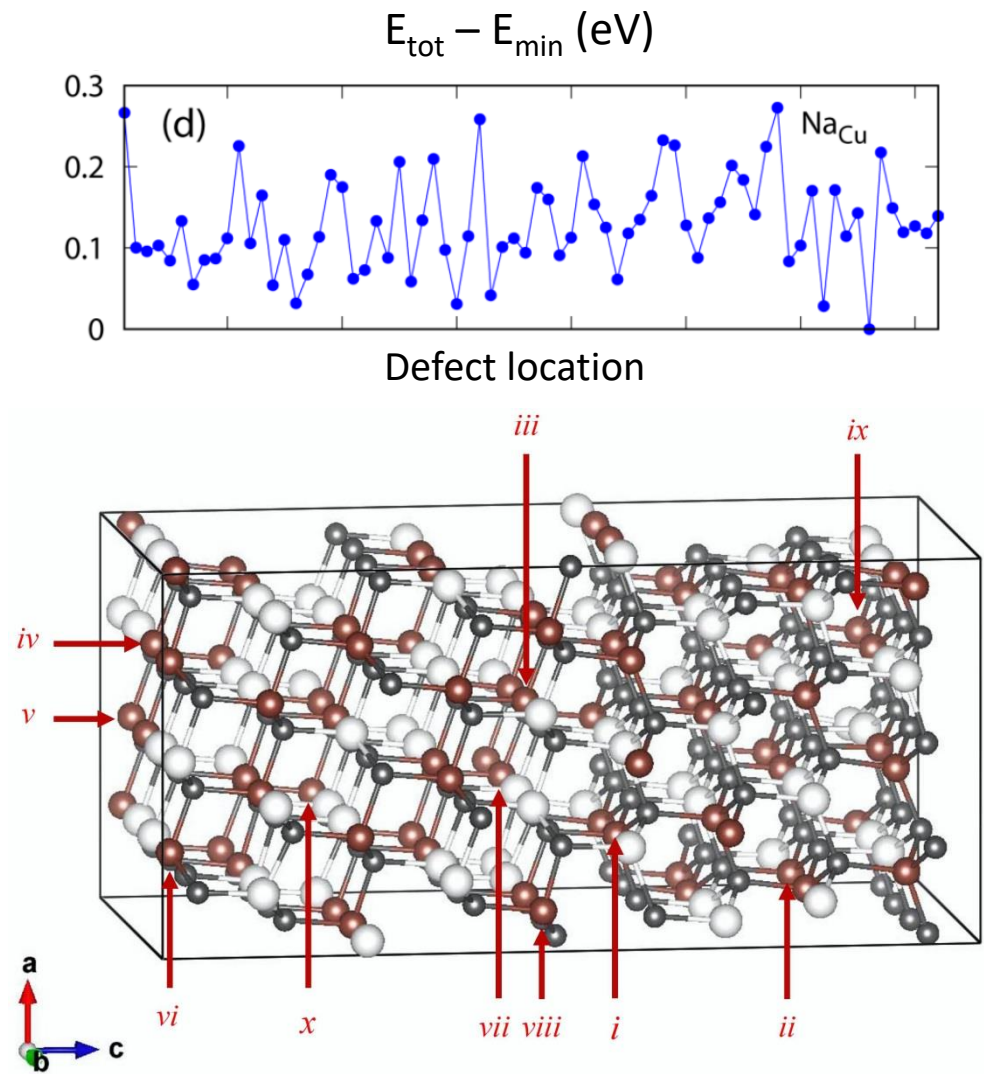

Upper panel: Total energies for  $\text{Na}_{\text{Cu}}$  at the different possible locations

Lower panel: Locations corresponding to the 10 lowest energy  $\text{Na}_{\text{Cu}}$  impurities

# Defect formation energies and equilibrium Fermi level self-consistently determined for monocrystalline CGS

Ga-rich conditions

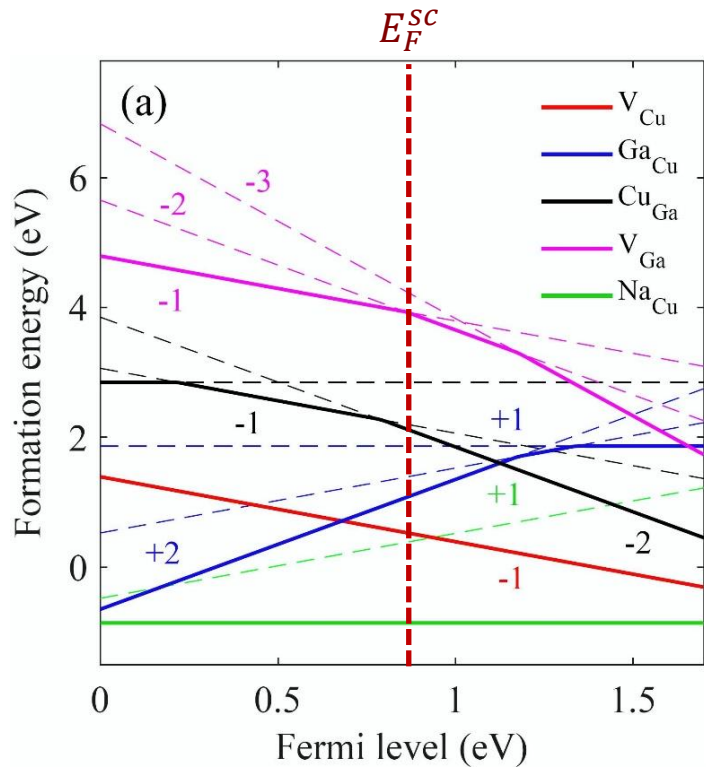

$$E_F^{sc} = 0.864 \text{ eV (without Na)}$$

Ga-poor conditions

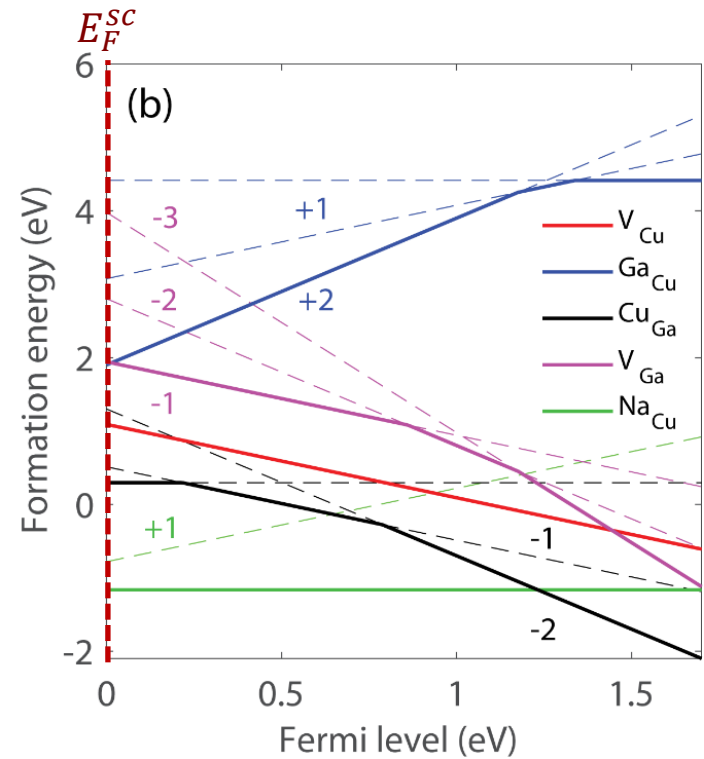

$$E_F^{sc} = 0 \text{ eV (without Na)}$$

(Note that  $E_F^{sc}$  is denoted  $E_F^{eq}$  in the main article)
